# Supplementary material for: Quantum networking with short-range entanglement assistance
Source: arXiv:2008.05553 ancillary file (2020-08-25)
Supplement: Supplementary file 1 [file Suppmat_qnet_shortentassist.pdf]

# Supplementary material for "Quantum networking with short-range entanglement assistance"

Siddhartha Santra and Vladimir S. Malinovsky
*US Army Research Laboratory, Adelphi, Maryland 20783, USA*

## STEPS FOR CATALYTIC ENTANGLEMENT CONCENTRATION

We first summarize the two steps needed to implement the transformation in Eq. (5) of the main text.

In step one, a temporary shared state $|\gamma(n,\alpha,c)\rangle$ which majorizes the initial state $|\alpha\rangle^{\otimes n}|\mathcal{C}\rangle$ is obtained with unit probability via operations on the joint state of qubits, $\{a_i\}_{i=1}^{i=(n+1)}$ and $\{b_i\}_{i=1}^{i=(n+1)}$, at $A$ and $B$, corresponding to a sequence of at most, $n_T \leq (2^{n+1}-1)$, T-transforms [2] (for example $n_T = 5$ for $n = 2$). The entries of $|\gamma(n,\alpha,c)\rangle$ are obtained algorithmically [3] from the set of ratios, $R_l(I,F), l \in [1, 2^{n+1}]$, and the entanglement monotones of the final state, $E_l(F)$, and are known to the agents at both $A$ and $B$. A circuit of depth $\sim 20n_T$ comprising of Toffoli, CNOT, single-qubit gates and single-qubit computational-basis measurements, implements the operations corresponding to the successive T-transforms on 2-dimensional subspaces of the $(n+1)$-qubit Hilbert space, $\otimes_{i=1}^{i=(n+1)}\mathcal{H}_{a_i}$, at node $A$. The set of measurement results is then conveyed as $n_T$-bits of classical data, $\bar{m}_A \in \{0,1\}^{n_T}$, to the agent at $B$ which determines the unitary it applies, $U_B(\alpha,c,\bar{m}_A)$. The latter can be implemented as a product of unitaries on the corresponding 2-dimensional subspaces of, $\otimes_{i=1}^{i=(n+1)}\mathcal{H}_{b_i}$, as a quantum circuit of depth $\sim 10n_T$ using the same set of basic gates. This completes the first step of deterministically obtaining $|\gamma(n,\alpha,c)\rangle$.

In step two, the agent at $B$ performs a two-outcome, $m_{1,2}$, set of generalized measurements, $M_{B,1}(\alpha,c)$ and $M_{B,2}(\alpha,c)$, on its portion of $|\gamma(n,\alpha,c)\rangle$ and obtains the state, $|\beta\rangle \otimes |00\rangle^{\otimes(n-1)} \otimes |\mathcal{C}\rangle$, if outcome $m_1$ is obtained - which occurs with probability, $P^{\max}_{\text{cat}}(n,\alpha,c)$. The success (or failure) of the transformation is then relayed to the agent at $A$ via a single-bit of classical communication. In case of success, agents at $A$ and $B$ can utilize the shared state $|\beta\rangle$ for entanglement swapping to extend its range (if the adjacent edges on either side also report success) and the catalyst state for further local entanglement concentration operations. Whereas, in case of failure they restart the process of generating $n$-copies of $|\alpha\rangle$ and reobtaining the catalyst state, $|\mathcal{C}\rangle$.

## OPERATIONS FOR CATALYTIC ENTANGLEMENT CONCENTRATION

Here we demonstrate the local operations required at the network nodes for catalytic entanglement concentration using $n = 2$ copies of the primary entangled states $\rho = |\alpha\rangle\langle\alpha|$ and one-copy of the optimal two-qubit catalyst state, $|\mathcal{C}_{\text{opt}}(2,\alpha)\rangle$, in Eq. (5) of the main text. We have derived the form of the optimal two-qubit catalyst for general '$n$' elsewhere [1], for $n = 2$ it is given by, $|\mathcal{C}_{\text{opt}}(2,\alpha)\rangle = \sqrt{c_0(2,\alpha)}\,|HV\rangle + \sqrt{1-c_0(2,\alpha)}\,|VH\rangle$, with, $c_0(2,\alpha) = (1+3\alpha^2-((1+3\alpha^2)^2-16\alpha^4)^{1/2})/4\alpha^2$. The form of the unitaries and measurement operators follow from results in [2],[3].

All operations at neighboring nodes $A, B$ are performed on two-dimensional subspaces of 3-qubits at each of the nodes. We use the Binary code for the tensor product basis of states on qubits $a_1, a_2, a_3$ and similarly for $b_1, b_2, b_3$, therefore,

$$\begin{aligned}
|000\rangle_{A_1A_2A_3} &\to |1\rangle_A\,, \\
|001\rangle_{A_1A_2A_3} &\to |2\rangle_A\,, \\
|010\rangle_{A_1A_2A_3} &\to |3\rangle_A\,, \\
|011\rangle_{A_1A_2A_3} &\to |4\rangle_A\,, \\
|100\rangle_{A_1A_2A_3} &\to |5\rangle_A\,, \\
|101\rangle_{A_1A_2A_3} &\to |6\rangle_A\,, \\
|110\rangle_{A_1A_2A_3} &\to |7\rangle_A\,, \\
|111\rangle_{A_1A_2A_3} &\to |8\rangle_A\,. 
\end{aligned} \tag{S1}$$

The state $|\alpha\rangle^{\otimes 2}|\mathcal{C}_{\text{opt}}(2,\alpha)\rangle$ in this basis is then given by the vector (suppressing the arguments of $c_0$ hereafter),

$$|I\rangle = |\alpha\rangle^{\otimes 2}|\mathcal{C}_{\text{opt}}(2,\alpha)\rangle = \begin{pmatrix} \sqrt{\alpha^2 c_0} \\ \sqrt{\alpha^2(1-c_0)} \\ \sqrt{\alpha(1-\alpha)c_0} \\ \sqrt{\alpha(1-\alpha)c_0} \\ \sqrt{\alpha(1-\alpha)(1-c_0)} \\ \sqrt{\alpha(1-\alpha)(1-c_0)} \\ \sqrt{(1-\alpha)^2 c_0} \\ \sqrt{(1-\alpha)^2(1-c_0)} \end{pmatrix}. \tag{S2}$$

The temporary state $|\gamma(2,\alpha,c_0(2,\alpha))\rangle$ is given by,

$$|\gamma\rangle = \begin{pmatrix} \sqrt{\alpha^2 c_0} \\ \sqrt{\alpha^2(1-c_0)} \\ \sqrt{(1-\alpha^2)/2} \\ \sqrt{(1-\alpha^2)/2} \\ 0 \\ 0 \\ 0 \\ 0 \end{pmatrix}, \tag{S3}$$

whose Schmidt coefficients majorize those of the initial state.

**STEP ONE**, as described in the main manuscript involves a sequence of 5 T-transforms to deterministically obtain $|\gamma\rangle$ from $|I\rangle$ via the following transformations,

$$|I\rangle \overset{T^{(1)}_{7-8}}{\to} |I_1\rangle \overset{T^{(2)}_{6-7}}{\to} |I_2\rangle \overset{T^{(3)}_{5-6}}{\to} |I_3\rangle \overset{T^{(4)}_{4-5}}{\to} |I_4\rangle \overset{T^{(5)}_{3-5}}{\to} |\gamma\rangle\,, \tag{S4}$$

where, the four intermediate states $|I_1\rangle \prec |I_2\rangle \prec |I_3\rangle \prec |I_4\rangle$ which sequentially majorize the preceding state are as follows:

$$\overset{|I_1\rangle}{\begin{pmatrix} \sqrt{\alpha^2 c_0} \\ \sqrt{\alpha^2(1-c_0)} \\ \sqrt{\alpha(1-\alpha)c_0} \\ \sqrt{\alpha(1-\alpha)c_0} \\ \sqrt{\alpha(1-\alpha)(1-c_0)} \\ \sqrt{\alpha(1-\alpha)(1-c_0)} \\ \sqrt{(1-\alpha)^2 c_0} \\ 0 \end{pmatrix}}, \overset{|I_2\rangle}{\begin{pmatrix} \sqrt{\alpha^2 c_0} \\ \sqrt{\alpha^2(1-c_0)} \\ \sqrt{\alpha(1-\alpha)c_0} \\ \sqrt{\alpha(1-\alpha)c_0} \\ \sqrt{\alpha(1-\alpha)(1-c_0)} \\ \sqrt{(1-\alpha c_0)(1-\alpha)} \\ 0 \\ 0 \end{pmatrix}}$$

$$\overset{|I_3\rangle}{\begin{pmatrix} \sqrt{\alpha^2 c_0} \\ \sqrt{\alpha^2(1-c_0)} \\ \sqrt{\alpha(1-\alpha)c_0} \\ \sqrt{\alpha(1-\alpha)c_0} \\ \sqrt{(1+\alpha-2\alpha c_0)(1-\alpha)} \\ 0 \\ 0 \\ 0 \end{pmatrix}}, \overset{|I_4\rangle}{\begin{pmatrix} \sqrt{\alpha^2 c_0} \\ \sqrt{\alpha^2(1-c_0)} \\ \sqrt{\alpha(1-\alpha)c_0} \\ \sqrt{(1-\alpha^2)/2} \\ \sqrt{(1+\alpha-2\alpha c_0)(1-\alpha)/2} \\ 0 \\ 0 \\ 0 \end{pmatrix}}. \tag{S5}$$

The $k$-th T-transform, $T_{i,j}^{(k)}$, involves unitaries and generalized measurements on the $2\times 2$ subspace $(|i\rangle_A, |j\rangle_A)$ of $\mathcal{H}^{a_1}\otimes\mathcal{H}^{a_2}\otimes\mathcal{H}^{a_3}$ and the corresponding subspace $(|i\rangle_B, |j\rangle_B)$ of $\mathcal{H}^{b_1}\otimes\mathcal{H}^{b_2}\otimes\mathcal{H}^{b_3}$. The transformation $|I\rangle \to |I_1\rangle$ is implemented using the following steps. First, Alice (agent at A) and Bob (agent at B) apply the local unitaries on the $\{|7\rangle_A, |8\rangle_A\}$ and $\{|7\rangle_B, |8\rangle_B\}$ subspaces respectively,

$$U_A^{(1)} = \begin{pmatrix} 1/\sqrt{2} & 1/\sqrt{2} \\ 1/\sqrt{2} & -1/\sqrt{2} \end{pmatrix},\ U_B^{(1)} = \begin{pmatrix} \sqrt{c_0} & \sqrt{1-c_0} \\ \sqrt{1-c_0} & -\sqrt{c_0} \end{pmatrix}. \tag{S6}$$

Alice then performs a generalized measurement using the following operators on the $\{|7\rangle_A, |8\rangle_A\}$ space,

$$M_{A,1}^{(1)} = \frac{\mathbb{1}_{A\setminus\{7,8\}}}{\sqrt{2}} \oplus |7\rangle_A\langle 7|,$$
$$M_{A,2}^{(1)} = \frac{\mathbb{1}_{A\setminus\{7,8\}}}{\sqrt{2}} \oplus |8\rangle_A\langle 8|, \tag{S7}$$

which form a complete set of measurements for Alice's systems since $(M_{A,1}^{(1)})^\dagger M_{A,1}^{(1)} + (M_{A,2}^{(1)})^\dagger M_{A,2}^{(1)} = \mathbb{1}_A$. The measurement result is then communicated to Bob who applies $\mathbb{1}_B$ in case Alice obtains $m_1^{(1)}$ and applies $\tilde{U}_B^{(1)}$ on the $\{|7\rangle_B, |8\rangle_B\}$ subspace if $m_2^{(1)}$ is obtained where (with $\cos\gamma_1 = (2c_0 - 1)$),

$$\tilde{U}_B^{(1)} = \begin{pmatrix} \cos\gamma_1 & \sin\gamma_1 \\ \sin\gamma_1 & -\cos\gamma_1 \end{pmatrix}. \tag{S8}$$

The transformation $|I_1\rangle \to |I_2\rangle$ is implemented similarly by first applying local unitary transforms at Alice and Bob's stations,

$$U_A^{(2)} = \begin{pmatrix} 1/\sqrt{2} & 1/\sqrt{2} \\ 1/\sqrt{2} & -1/\sqrt{2} \end{pmatrix},\ U_B^{(2)} = \begin{pmatrix} \sqrt{s} & \sqrt{1-s} \\ \sqrt{1-s} & -\sqrt{s} \end{pmatrix} \tag{S9}$$

with $s = \alpha(1-c_0)/(1-\alpha c_0)$. This is followed by the measurement of local operators by Alice,

$$M_{A,1}^{(2)} = \frac{\mathbb{1}_{A\setminus\{6,7\}}}{\sqrt{2}} \oplus |6\rangle_A\langle 6|,$$
$$M_{A,2}^{(2)} = \frac{\mathbb{1}_{A\setminus\{6,7\}}}{\sqrt{2}} \oplus |7\rangle_A\langle 7|, \tag{S10}$$

and the measurement results communicated to Bob. If Alice obtains $m_1^{(2)}$ Bob applies $\mathbb{1}_B$ and if Alice obtains $m_2^{(2)}$ then Bob applies (with $\cos\gamma_2 = (2\alpha - (1+\alpha c_0))/(1-\alpha c_0)$),

$$\tilde{U}_B^{(2)} = \begin{pmatrix} \cos\gamma_2 & \sin\gamma_2 \\ \sin\gamma_2 & -\cos\gamma_2 \end{pmatrix}. \tag{S11}$$

The transformation $|I_2\rangle \to |I_3\rangle$ is implemented similarly by first applying local unitary transforms at Alice and Bob's stations,

$$U_A^{(3)} = \begin{pmatrix} 1/\sqrt{2} & 1/\sqrt{2} \\ 1/\sqrt{2} & -1/\sqrt{2} \end{pmatrix},\ U_B^{(3)} = \begin{pmatrix} \sqrt{s} & \sqrt{1-s} \\ \sqrt{1-s} & -\sqrt{s} \end{pmatrix}, \tag{S12}$$

with $s = \alpha(1-c_0)/(1+\alpha-2\alpha c_0)$. This is followed by the measurement of local operators by Alice,

$$M_{A,1}^{(3)} = \frac{\mathbb{1}_{A\setminus\{5,6\}}}{\sqrt{2}} \oplus |5\rangle_A\langle 5|,$$
$$M_{A,1}^{(3)} = \frac{\mathbb{1}_{A\setminus\{5,6\}}}{\sqrt{2}} \oplus |6\rangle_A\langle 6|, \tag{S13}$$

and the measurement results communicated to Bob. If Alice obtains $m_1^{(3)}$ Bob applies $\mathbb{1}_B$ and if Alice obtains $m_2^{(3)}$ then Bob applies (with $\cos\gamma_3 = (\alpha-1)/(1+\alpha-2\alpha c_0)$),

$$\tilde{U}_B^{(3)} = \begin{pmatrix} \cos\gamma_3 & \sin\gamma_3 \\ \sin\gamma_3 & -\cos\gamma_3 \end{pmatrix}. \tag{S14}$$

The transformation $|I_3\rangle \to |I_4\rangle$ is implemented similarly by first applying local unitary transforms at Alice and Bob's stations,

$$U_A^{(4)} = \begin{pmatrix} 1/\sqrt{2} & 1/\sqrt{2} \\ 1/\sqrt{2} & -1/\sqrt{2} \end{pmatrix},\ U_B^{(4)} = \begin{pmatrix} \sqrt{s} & \sqrt{1-s} \\ \sqrt{1-s} & -\sqrt{s} \end{pmatrix}, \tag{S15}$$

with $s = \alpha c/(1+\alpha-\alpha c)$. This is followed by the measurement of local operators by Alice,

$$M_{A,1}^{(4)} = \frac{\mathbb{1}_{A\setminus\{4,5\}}}{\sqrt{2}} \oplus \cos\delta\,|4\rangle_A\langle 4| + \sin\delta\,|5\rangle_A\langle 5|,$$
$$M_{A,2}^{(4)} = \frac{\mathbb{1}_{A\setminus\{4,5\}}}{\sqrt{2}} \oplus \sin\delta\,|4\rangle_A\langle 4| + \cos\delta\,|5\rangle_A\langle 5|, \tag{S16}$$

with $\cos\delta = (0.5+0.5\sqrt{(4\alpha c_0 - (1+\alpha))/(4\alpha c_0)})^{1/2}$ and the measurement results communicated to Bob. If Alice obtains $m_1^{(4)}$ Bob applies $\mathbb{1}_B$ and if Alice obtains $m_2^{(4)}$ then Bob applies (with $\cos\gamma_4 = (3\alpha c_0 - 1 - \alpha)/(1+\alpha-\alpha c_0)$),

$$\tilde{U}_B^{(4)} = \begin{pmatrix} \cos\gamma_4 & \sin\gamma_4 \\ \sin\gamma_4 & -\cos\gamma_4 \end{pmatrix}. \tag{S17}$$

Next, the transformation $|I_4\rangle \to |\gamma_1\rangle$ is implemented by first applying local unitary transforms at Alice and Bob's stations,

$$U_A^{(5)} = \begin{pmatrix} 1/\sqrt{2} & 1/\sqrt{2} \\ 1/\sqrt{2} & -1/\sqrt{2} \end{pmatrix}, \; U_B^{(5)} = \begin{pmatrix} \sqrt{s} & \sqrt{1-s} \\ \sqrt{1-s} & -\sqrt{s} \end{pmatrix}, \quad \text{(S18)}$$

with $s = 2\alpha c_0/(1+\alpha)$. This is followed by the measurement of local operators by Alice,

$$M_{A,1}^{(5)} = \frac{\mathbb{1}_{A\backslash\{3,5\}}}{\sqrt{2}} \oplus |3\rangle_A \langle 3|,$$
$$M_{A,2}^{(5)} = \frac{\mathbb{1}_{A\backslash\{3,5\}}}{\sqrt{2}} \oplus |5\rangle_A \langle 5|, \quad \text{(S19)}$$

and the measurement results communicated to Bob. If Alice obtains $m_1^{(5)}$ Bob applies $\mathbb{1}_B$ and if Alice obtains $m_2^{(5)}$ then Bob applies (with $\cos\gamma_5 = ((4\alpha c_0)/(1+\alpha)-1)$),

$$\tilde{U}_B^{(5)} = \begin{pmatrix} \cos\gamma_5 & \sin\gamma_5 \\ \sin\gamma_5 & -\cos\gamma_5 \end{pmatrix}. \quad \text{(S20)}$$

This completes the process of deterministically obtaining the shared state $|\gamma\rangle$ between $A$ and $B$ using local operations and multiple rounds of one-way classical communication.

The sequence of operations (S6)-(S20) can, however, be equivalently performed by completing all operations on Alice's side first and then communicating 5-bits of classical data to Bob which determines the unitary that Bob applies. For this, the generalized measurements (S7), (S10), (S13), (S16), (S19) are performed by unitarily interacting qubits $a_1, a_2, a_3$ with measurement qubits $q^{(i)}$, initialized in the $|0\rangle$ state, via unitaries $U_{A,M}^{(i)}$ respectively, where

$$U_{A,M}^{(1)} = \frac{\mathbb{1}_{A\backslash\{7,8\}}}{\sqrt{2}} \otimes (HX) + |7\rangle\langle 7| \otimes \mathbb{1} + |8\rangle\langle 8| \otimes iY, \quad \text{(S21)}$$

$$U_{A,M}^{(2)} = \frac{\mathbb{1}_{A\backslash\{6,7\}}}{\sqrt{2}} \otimes (HX) + |6\rangle\langle 6| \otimes \mathbb{1} + |7\rangle\langle 7| \otimes iY, \quad \text{(S22)}$$

$$U_{A,M}^{(3)} = \frac{\mathbb{1}_{A\backslash\{5,6\}}}{\sqrt{2}} \otimes (HX) + |5\rangle\langle 5| \otimes \mathbb{1} + |6\rangle\langle 6| \otimes iY, \quad \text{(S23)}$$

$$U_{A,M}^{(4)} = \frac{\mathbb{1}_{A\backslash\{4,5\}}}{\sqrt{2}} \otimes (HX) + |4\rangle\langle 4| \otimes (\cos\delta\mathbb{1} + \sin(\delta) iY)$$
$$+ |5\rangle\langle 5| \otimes (\sin\delta\mathbb{1} + \cos(\delta) iY), \quad \text{(S24)}$$

$$U_{A,M}^{(5)} = \frac{\mathbb{1}_{A\backslash\{3,5\}}}{\sqrt{2}} \otimes (HX) + |3\rangle\langle 3| \otimes \mathbb{1} + |5\rangle\langle 5| \otimes iY, \quad \text{(S25)}$$

where $\cos\delta = (0.5 + 0.5\sqrt{(4\alpha c_0 - (1+\alpha))/(4\alpha c_0)})^{1/2}$. The measurement qubits are then measured in the computational basis to obtain 5-bits of classical data, $\bar{m}_A \in \{0,1\}^5$. The complete sequence of unitaries applied by Alice is therefore (with the earlier unitary, i.e. with smaller '$i$', to the right),

$$\prod_{i=1}^{i=5} U_{A,M}^{(i)} U_A^{(i)}. \quad \text{(S26)}$$

The 5-bits of classical data is then conveyed to Bob which determines the unitary that it applies to qubits $b_1, b_2, b_3$,

$$U_B(\alpha, c, \bar{m}_A) = \prod_{i=1}^{i=5} (\tilde{U}_B^{(i)})^{m_{A,i}} U_B^{(i)}. \quad \text{(S27)}$$

The quantum circuit for each pair of unitaries $U_{A,M}^{(i)} U_A^{(i)}$ in expression (S26) has an approximate depth of 20. We provide, as an example, a possible circuit to implement $U_{A,M}^{(4)}$:

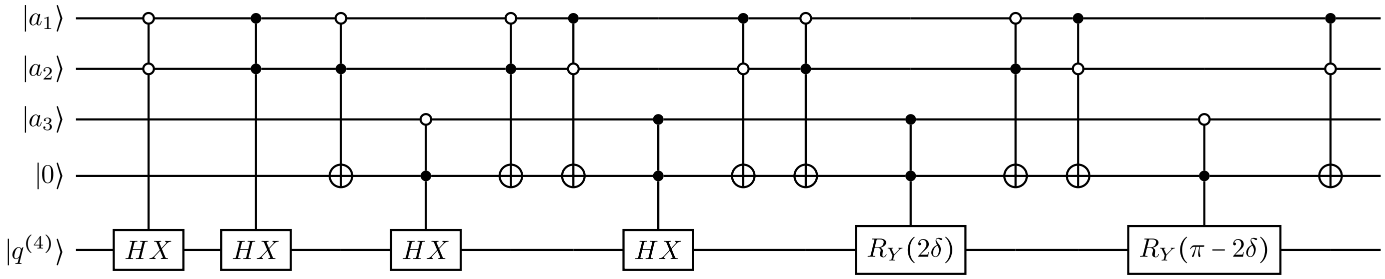


**STEP TWO** as described in the main manuscript involves Bob measuring the operators on qubits $b_1, b_2, b_3$,

$$M_{B,1} = \cos\kappa_1 |1\rangle_B \langle 1| + \cos\kappa_2 |2\rangle_B \langle 2| + \mathbb{1}_{A\backslash\{1,2\}},$$
$$M_{B,2} = \sin\kappa_1 |1\rangle_B \langle 1| + \sin\kappa_2 |2\rangle_B \langle 2| \quad \text{(S28)}$$

where, $\cos\kappa_1 = \sqrt{(1-\alpha^2)/(2\alpha^2(1-c_0))}$ and $\cos\kappa_2 = \sqrt{(c_0(1-\alpha^2))/(2\alpha^2(1-c_0)^2)}$. If the outcome of Bob's measurement is $m_1$ corresponding to $M_{B,1}$, then they obtain the post-measurement state $|\beta\rangle \otimes |\mathcal{C}_0\rangle \otimes |HV\rangle$ with probability, $P(\alpha) = (1-\alpha^2)/(1-c_0(2,\alpha))$. On the other hand, if Bob obtains $m_2$ then the attempt has been a failure. In either case the outcome is conveyed to Alice so that subsequent actions for long-range entanglement distribution can continue.

[1] S. Santra and V. S. Malinovsky, arXiv:2007.10516.
[2] M. A. Nielsen, Phys. Rev. Lett. **83**, 436 (1999).
[3] G. Vidal, Phys. Rev. Lett. **83**, 1046 (1999).
